# Supplementary material for: Assessing Neural Network Robustness via Adversarial Pivotal Tuning
Source: arXiv:2211.09782 source file (2024-01-06)
Supplement: Supplementary file 1 [file Appendix.tex]

\section{Implementation Details}

\subsection{APT details}
For the latent optimizaton step 
(\cref{eq:inversion}), we use the hyperparameters described by \cite{karras2020analyzing}. We run the optimization for $1k$ iterations. 

We use a linear learning rate scheduler for 50 iterations starting with a learning rate of 0 and ending with a maximum learning rate of $0.05$. 

Afterwards we use a cosine scheduler for the last 250 iterations that is ramped  down to 0.

Our StyleGAN-XL generated images are of $256^2$ resolution. Given a generated image, 
we follow \cite{PRIME2021} in center cropping the image to $224^2$ and resolution and normalising it using standard ImageNet statistics, before being classified by our pretrained classifier. 

The hyperparameters in Eq.~\ref{eq:loss} are: $\lambda_{L2}^P = \lambda_{L2}^R = 0.1$, $\lambda_{CE}=0.01$ and $\lambda_{PG}=0.005$.

For \cref{eq:loss}, we use the Adam optimiser with a learning rate of $3e-4$. 

When fintuning on APT generated images, we follow our standard training configuration, but lower the learning rate to  $0.001$. 

\subsection{PGD and SSAH details}
We follow \cite{madry2017towards} for standard hyperparameter except that we use 40 iterations.
For SSAH \cite{luo2022frequency} we also follow the standard hyperparameters but use 200 iterations.

\subsection{Model details}

We use the model weights for PRIME-Resnet50~\cite{PRIME2021} and FAN-VIT~\cite{zhou2022understanding} from their original repositories.

Models in \cref{tab:transfer-study} and Tab.~\ref{tab:new} are chosen due to their diverse architectures and their availability on \texttt{torchvision}.

We use the large CLIP model in Section 4.3 for evaluating the similarity among the images in \cref{fig:component_examples}
